# Supplementary material for: Sycophancy Mitigation Through Reinforcement Learning with Uncertainty-Aware Adaptive Reasoning Trajectories
Source: arXiv:2509.16742 source file (2025-09-20)
Supplement: Supplementary file 1 [file detail.tex]

\subsection{Implementation Details}
\label{app: details}
